# Supplementary material for: Predicting Exoplanets Mass and Radius: A Nonparametric Approach
Source: arXiv:1811.02324 source file (2018-11-06)
Supplement: Supplementary file 1 [file Appendix-CV.tex]

\section{Cross validation}
\label{sec:cv}

We use 10-fold cross validation to choose the optimal value of degrees $d$ in
(\ref{bernMod-C}).
We separate the dataset randomly into 10 folds, 
within each fold, the number of observation are similar. 
We leave each fold out and fit the rest 9 folds sequentially into the model,
then 10 estimated weights will be obtained. 
We denote the estimated weight using 
data in $1, \dots, s-1, s+1, \dots, 10$ folds to be $\hat{\boldsymbol w}^{(s)}$.
We then plug-in each $\hat{\boldsymbol w}^{(s)}$ along with the data 
in the $s$-th fold to calculate the predicted log-likelihood.
The predicted log-likelihood has the expression as follows,
by obtaining $\boldsymbol c_s$ which defined in Appendix \ref{sec:maxlikderive}
using data in $s$-th fold, then
we have 
\begin{equation}
	\log L^{\text{pred}} 
	= 
	\sum_{i=1}^{10} \log(\hat{\boldsymbol w}^{(s) T} \boldsymbol c_s).
\end{equation}
We calculate $\log L^{\text{pred}}$ for different possible values of $d$,
and choose the one gives the largest value of $\log L^{\text{pred}}$.
