# Supplementary material for: Predicting Exoplanets Mass and Radius: A Nonparametric Approach
Source: arXiv:1811.02324 source file (2018-11-06)
Supplement: Supplementary file 2 [file Appendix-MLE.tex]

\section{MLE for Bernstein Polynomials method}
\label{sec:maxlikderive}

This appendix gives details of using an MLE method to inference the
model (\ref{bernMod-A})-(\ref{bernMod-C}) in Section \ref{sec:model}.

The likelihood can be written as
\begin{equation}
\label{equ-apx-A1}
\begin{split}
	L(\boldsymbol w| & \boldsymbol M^{\text{obs}}, 
										\boldsymbol R^{\text{obs}}, 
										\boldsymbol \sigma^{{\text{obs}}}_{M}, 
										\boldsymbol \sigma^{{\text{obs}}}_{R})\\
 	& =
    \int_{\underline{M}}^{ \overline{M}} 
    \int_{\underline{R}}^{ \overline{R}} 
	f(\boldsymbol M^{\text{obs}}, 
	  \boldsymbol R^{\text{obs}}, m, r | 
		\boldsymbol w, 
		\boldsymbol \sigma^{{\text{obs}}}_M, 
		\boldsymbol \sigma^{{\text{obs}}}_R)
	\ \text{d}r \text{d}m \\
  	& = 
	\prod_{i=1}^n     
	\int_{\underline{M}}^{ \overline{M}} 
    \int_{\underline{R}}^{ \overline{R}} 
	f(M^{\text{obs}}_i| m, \sigma^{{\text{obs}}}_{M_i}) 
    f(R^{\text{obs}}_i| r,  \sigma^{{\text{obs}}}_{R_i}) 
    f(m, r| \boldsymbol w) 
     \ \text{d}r \text{d}m\\
	& = 
	\prod_{i=1}^n \sum_{k=1}^{d} \sum_{l=1}^{d} w_{kl}
	\int_{\underline{M}}^{ \overline{M}}  
				\frac{1}{\sigma_{M, i}^{\text{obs}}}
				\mathcal{N} \Big (\frac{M_i^{\text{obs}} - m}{\sigma_{M_i}^{\text{obs}}} \Big )
				\frac{\beta_k(\frac{m - \underline{M}}{\overline{M} - \underline{M}})}{\overline{M} - \underline{M}} 
				\ \text{d}m \\
	& \quad \quad \quad \quad \quad \quad \
			\times 
			\int_{\underline{R}}^{ \overline{R}} \frac{1}{\sigma_{R, i}^{\text{obs}}}
			\mathcal{N} \Big(\frac{R_i^{\text{obs}} - r}{\sigma_{R_i}^{\text{obs}}} \Big)
		   \frac{\beta_l(\frac{r - \underline{R}}{\overline{R} - \underline{R}})}{\overline{R}-\underline{R}}
		   \ \text{d}r.
\end{split}
\end{equation}

We let
\begin{equation*}
c_{kl,i} \equiv
	\int_{\underline{M}}^{ \overline{M}} 
	\frac{1}{\sigma_{M_i}^{\text{obs}}}
				\mathcal{N} \Big (\frac{M_i^{\text{obs}} - m}{\sigma_{M_i}^{\text{obs}}} \Big )
				\frac{\beta_k(\frac{m - \underline{M}}{\overline{M} - \underline{M}})}{\overline{M} - \underline{M}} 
				\ \text{d}m
	\int_{\underline{R}}^{\overline{R}} 
	\frac{1}{\sigma_{R_i}^{\text{obs}}}
	\mathcal{N} \Big(\frac{R_i^{\text{obs}} - r}{\sigma_{R_i}^{\text{obs}}} \Big)
    \frac{\beta_l(\frac{r - \underline{R}}{\overline{R} - \underline{R}})}{\overline{R}-\underline{R}}
    \ \text{d}r,
\end{equation*}
and this is a product of two constants,
the integration can be calculate numerically such as using the 
``integrate()'' function in $\mathsf{R}$.
